# Supplementary material for: Progressive Localization Networks for Language-based Moment Localization
Source: arXiv:2102.01282 source file (2022-03-03)
Supplement: Supplementary file 1 [file appendix.tex]

{

\begin{figure}[tb!]
\centering
\subfigure[on TACoS]{
\includegraphics[width=0.99\linewidth]{figure/score_map_tacos}
}
\quad
\subfigure[on ActivityNet Captions]{
\includegraphics[width=0.99\linewidth]{figure/scores_map_acnet23}
}
\caption{Two examples of language-based moment localization by our model on (a) TACoS, (b) ActivityNet Captions. 
  For each query and the corresponding video, we illustrate the predicted score maps of PLN$_{2,1}$ and PLN$_{2,2}$, where red boxes indicate target moments and blue boxes indicate top-1 predicted moments. PLN$_{2,1}$ indicates our proposed two-stage PLN using the predicted score map of stage 1 for prediction, while PLN$_{2,2}$ is the same two-stage model but uses the output of stage 2.
  The later stage of PLN gives more accurate localization.  Best viewed in zoom in.
  }\label{fig:score_map_more}
\end{figure}

\section{The Influence of the number of stages}\label{app:stage}

\begin{table*}[htb!]
\caption{Performance of PLN with the different number of stages on the ActivityNet Captions dataset and Charades-STA dataset.}
\label{tab:multi_stage_ac_cha}
\centering
\scalebox{0.7}{
\begin{threeparttable}
\begin{tabular}{@{}l*{19}{c} @{}}
\toprule
\multirow{3}{*}{\textbf{Method}} &
%   \multirow{3}{*}{\textbf{Source}} &
  \multicolumn{8}{c}{\textbf{ActivityNet}} &&
  \multicolumn{8}{c}{\textbf{Charades-STA}} &
   \\ \cmidrule{2-9} \cmidrule{11-18}
   &
  \multicolumn{3}{c}{\textbf{Rank@1,IoU=m}} &&
  \multicolumn{3}{c}{\textbf{Rank@5,IoU=m}} &
  \multirow{2}{*}{\textbf{mIoU}} &&
  \multicolumn{3}{c}{\textbf{Rank@1,IoU=m}} &&
  \multicolumn{3}{c}{\textbf{Rank@5,IoU=m}} &
  \multirow{2}{*}{\textbf{mIoU}} & \\ \cmidrule{2-4} \cmidrule{6-8} \cmidrule{11-13} \cmidrule{15-17}
         &                  0.3   & 0.5   & 0.7   && 0.3   & 0.5   & 0.7   &&      & 0.3   & 0.5   & 0.7   && 0.3   & 0.5   & 0.7   &       &  \\ 
\midrule
\textbf{one-stage:}   &  &  & & & & & &  \\
$N^t$=8   &59.03  &43.05  &25.78 &&85.13 &75.79 &55.66 &42.96  && 63.23  & 48.15  & 26.84 &&\textbf{97.98} & 97.07 & 46.75 & 43.05\\

$N^t$=16         & 59.75  & 43.32  & 25.81 &&85.46 & 75.96 & 59.98 & 42.89 && 61.64  & 48.90  & 28.92 &&96.48 & 86.77 & 52.28 & 43.45 \\

$N^t$=32         & 58.14  & 42.40  & 24.99 &&85.27 & 76.34 & 60.66 & 42.22 && 63.63  & 52.34  & 30.65 &&97.15 & 88.71 & 56.19 & 44.54 \\

$N^t$=64         & 57.45  & 40.87  & 23.04 &&85.22 & 74.89 & 57.89 & 41.00 && 67.07  & 52.74  & 28.90 &&97.23 & 89.49 & 56.61 & 45.78 \\

\hline
\textbf{two-stage:}   &  &  & & & & & &  \\
$N^t$=16-64       & 59.65 & \textbf{45.66}  & \textbf{29.28} && \textbf{85.66}  & 76.65  & \textbf{63.06} & 44.12  && 68.60   & 56.02   & \textbf{35.16}  &   & 94.54 & 87.63 & \textbf{62.34} & \textbf{49.09} \\

\hline
\textbf{three-stage:}   &  &  & & & & & &  \\
$N^t$=16-32-64    & \textbf{61.58} & 45.58 & 27.25 && 85.35 & \textbf{76.96} & 61.93 & \textbf{44.22}  && \textbf{69.25}  & \textbf{57.07} & 35.00 && 96.85 & \textbf{89.60} & 59.06  & 48.84 \\

\hline
\textbf{four-stage:}   &  &  & & & & & &  \\
$N^t$=8-16-32-64  &60.06 & 45.43 & 28.72 && 84.92  & 76.03 & 60.31  & 43.85 && 68.20 & 54.41 & 31.72  && 96.53 & 89.27  & 57.90  & 47.28   \\ 

\bottomrule
\end{tabular}

\end{threeparttable}
}
\end{table*}

Here, we evaluate the performance of PLN variants with the different number of stages on ActivityNet Captions and Charades-STA.
As shown in Table \ref{tab:multi_stage_ac_cha}, the models with multiple stages again outperform the one-stage counterparts.
Additionally, different from the result that the two-stage one turns out to be better than the three-stage and four-stage models on TACoS, their performance is comparable on ActivityNet Captions and Charades-STA.
We conjecture this is due to the fact that TACoS has much fewer training videos than ActivityNet Captions and Charades-STA (See Table \ref{tab:dataset_statistics}). 
On the whole, the two-stage PLN achieves the best overall performance on the three datasets.

\begin{table}[htb!]

\caption{The average length of top-5 predicted moments in different stages of our proposed two-stage PLN. The unit of the video length is seconds. }
\label{tab:coarse_to_fine}
\centering
\scalebox{0.8}{
\begin{tabular}{lcc}
\toprule
\textbf{Dataset}   & \textbf{First stage}  &  \textbf{Second stage}    \\ 
\midrule
\textbf{TACoS}                & 39.54 & 38.86  \\
\textbf{ActivityNet Captions} & 44.85 & 42.31  \\
\textbf{Charades-STA}         & 8.57  & 7.71    \\ 
\bottomrule
\end{tabular}
}
\end{table}

\section{Analysis on lengths of predicted moments in different stages}
In this section, we explore the lengths of predicted moments in different stages.
Specifically, we measure the average length of top-5 predicted moments in different stages of our proposed two-stage PLN. The results on TACoS, ActivityNet Captions and Charades-STA are summarized in Table  \ref{tab:coarse_to_fine}. On the three datasets, the average length of predicted moments obtained via the second stage is consistently shorter than that obtained via the first stage.
The result to some extent verifies that the localization branch in the early stage focuses on the moments generated with the clips of large temporal granularity, while the later localization branch focuses more on the moments generated with the clips of a small granularity.

\begin{table}[tb!]
% \vspace{0.1in}
\caption{ The influence of relevance score prediction  module.}
  \label{tab:relevance_score}
%   \vspace{-0.1in}
 %\renewcommand{\arraystretch}{0.7}
  \centering
\scalebox{0.8}{%
\begin{threeparttable}
    \begin{tabular}{@{}ll*{6}{c} @{}} 
     \toprule
      \multirow{2}{*}{ \textbf{Dataset}} &
      \multirow{2}{*}{ \textbf{Score Prediction}} &
      \multicolumn{3}{c}{ \textbf{Rank@1,IoU=m}} &
      \multirow{2}{*}{ \textbf{mIoU}} \\
      \cmidrule{3-5} 
      &&  0.3   &  0.5   &  0.7   &         \\ 
      \midrule
      \multirow{2}{*}{ \textbf{Charades-STA}}
      &  ConvNet          &  \textbf{59.33} &  \textbf{45.43} &  \textbf{26.26}  &  \textbf{41.28} \\
    %   & scale dot (both)             & 57.50 & 44.09 & 25.89       &  40.19     \\
    %   & ConvNet+DP           & 56.32 & 42.28 & 24.01       &  38.53     \\
      &  Dot product          &  56.96 &  40.83 &  20.62   &  38.20     \\
      \midrule
       \multirow{2}{*}{ \textbf{TACoS}}
      &  ConvNet          &  \textbf{43.89} &  \textbf{31.12} &  \textbf{16.10}  &  \textbf{29.70}\\
    %   & scale dot (both)               & 39.04 & 24.99 & 11.70       &  25.72   \\
    %   & ConvNet+DP             & 38.42 & 25.47 & 13.12       &  25.83     \\
      &  Dot product           & 34.14 & 20.12 &  11.55       & 22.94     \\
     \midrule
      
    \multirow{2}{*}{ \textbf{ActivityNet Captions}}
      &  ConvNet          &  \textbf{59.65} &  \textbf{45.66} &  \textbf{29.28}  &  \textbf{44.12}\\
    %   & scale dot (both)               &\textbf{59.95} & 45.33 & 28.17   & 43.68    \\
    %   &ConvNet+DP              & 59.81 & 44.80 & 27.12       &  43.28     \\
      &  Dot product           &  59.61 &  41.12 &  22.82       &   41.70     \\
     
      %\hline
      \bottomrule
    \end{tabular}%
    \end{threeparttable}
 }
%   \vspace{-0.1in}
  
\end{table}

\section{The Influence of Relevance Score Prediction}\label{app:relevance}
Recall that in our proposed model we first fuse candidate moments and a given sentence query by an element-wise multiplication, and further employ a ConvNet that consists of two stacked convolutional layers and an FC layer to predict relevance scores.
To explore its effectiveness for relevance score prediction, we compare it with a common method, \ie dot product between the features of candidate moments and the query features.
As shown in Table \ref{tab:relevance_score}, ConvNet consistently outperforms the dot product. We attribute the better performance of ConvNet to that it models the dependencies between candidate moments thus enables the network to perceive more context information from the adjacent candidate moments. By contrast, dot product matches the query with moment candidates independently, which ignores the moment dependencies.

}
